# Supplementary material for: QuickDrop: Efficient Federated Unlearning by Integrated Dataset Distillation
Source: arXiv:2311.15603 source file (2024-12-06)
Supplement: Supplementary file 1 [file appendix_discussion.tex]

\section{Executing Multiple Unlearning Requests in Parallel}
\label{subsec:parallel_unlearning_requests}
In~\Cref{subsec:exp_sequential_unlearning}, we have demonstrated how \sys is able to execute subsequent, multiple unlearning requests for different classes.
While we assume in this experiment that unlearning requests are processed one-by-one, batching multiple unlearning requests could save time and compute resources.
\sys supports the processing of multiple unlearning requests at the same time by having clients execute \sga using the distilled data representing the samples being unlearned, and then execute the recovery stage with the distilled data representing the remaining data.
This enables the network to unlearn multiple classes, or the data of multiple clients using a single unlearning and recovery stage.
%Advanced scheduling algorithms could be a future avenues to explore to implement batching of unlearning requests effectively.
